# Supplementary material for: Asymmetric enzyme kinetics of F1-ATPase induced by rotation-assisted substrate binding
Source: arXiv:2402.17326 source file (2025-05-21)
Supplement: Supplementary file 1 [file si.pdf]

# Supplemental Material for “Bypass mechanism of F<sub>1</sub>-ATPase for asymmetric enzyme kinetics”

Yohei Nakayama<sup>1</sup> and Shoichi Toyabe<sup>1</sup>

<sup>1</sup>*Department of Applied Physics, Graduate School of Engineering,  
Tohoku University, Aoba 6-6-05, Sendai 980-8579, Japan*

## I. MATERIALS AND METHODS

### A. Preparation of F<sub>1</sub>

$\alpha_3\beta_3\gamma$  subcomplexes of F<sub>1</sub> derived from a thermophilic *Bacillus* PS3 with mutations for the rotation assay (His<sub>6</sub>- $\alpha$ C193S/W463F, His<sub>10</sub>- $\beta$ , and  $\gamma$ S107C/I210C) [1] were expressed and purified in the same way as [2], except that the treatment with ( $\pm$ )-dithiothreitol before flash freezing was omitted.

### B. Ni<sup>2+</sup>-NTA modification of cover glasses

In our single-molecule experiments, F<sub>1</sub> molecules were adhered to a cover glass modified by Ni<sup>2+</sup>-NTA. The Ni<sup>2+</sup>-NTA glass was prepared as follows. Cover glasses (24 × 36mm<sup>2</sup> or 24 × 32mm<sup>2</sup>, thickness No. 1; Matsunami) were washed with ultrapure water three times and immersed in 10 M potassium hydroxide solution overnight. The glasses were washed with RO water five times and ultrapure water one time, and immersed in a 1:1 mixture of ethanol and ultrapure water containing 2 % v/v (3-Mercaptopropyl)trimethoxysilane (purchased from TCI, Japan) and 0.06 % v/v acetic acid for 120 min at 60 °C. They were washed with ultrapure water three times, and baked at 120 °C for 60 min. They were immersed in 50 mM phosphate buffer (pH 6.7) containing 1 mM ( $\pm$ )-dithiothreitol and 2 mM ethylenediaminetetraacetic acid for 90 min. They were washed with RO water five times and ultrapure water one time, and reacted with 1.8 mg/ml Maleimido-C<sub>3</sub>-NTA (purchased from Dojindo, Japan) in 100 mM phosphate buffer (pH 6.7) for 60 min. The glasses were immersed in 50 mM nickel sulfate solution for 30 min, and washed with RO water five times and ultrapure water one time, before using them for single-molecule experiments.

### C. Single-molecule experiments

The experimental setup is essentially the same as that in the previous study [2]. An observation chamber consisted of a Ni<sup>2+</sup>-NTA modified cover glass and a slide with quadrupolar electrodes. The cover glass and the slide were separated by double-sided adhesive tape (10  $\mu$ m thickness; Teraoka, 7070W) with silicone grease (Shin-Etsu Chemical, Japan) on a surface. The solution of F<sub>1</sub> was diluted with 50 mM MOPS buffer (pH 6.7) containing 5 mg/ml bovine serum albumin, 50 mM potassium chloride, and 1 mM magnesium chloride (buffer II) to a final concentration of 1 nM. The chamber was filled with the solution, and incubated for 10 min to immobilize F<sub>1</sub> molecules on the surfaces. The bovine serum albumin was added as the blocking agent. The chamber was washed with buffer II, and streptavidin-coated polystyrene particles (diameter = 276 nm, Thermo Fisher Scientific) diluted with buffer II was infused into it. Azide contained in the solution of polystyrene particle was removed in advance by repeating centrifugation, exchange of supernatant, and re-dispersion six times. After a 30 min incubation, the solution in the chamber was exchanged with 5 mM MOPS and 1 mM phosphate buffer containing 1 mM magnesium chloride, and indicated amount of MgATP and MgADP (pH 7.0).

Rotation of the  $\gamma$ -shaft was probed by dimeric polystyrene particles attached to the biotinylated  $\gamma$ -shaft. The observation was performed on a bright-field upright microscope (Olympus, Japan) with a 100× objective (NA1.40), high-intensity LED (623 nm, 4.8 W, Thorlabs, NJ) for illumination, a high-speed camera (Basler, Germany) at 4,000 Hz, and a laboratory-made capturing software developed on LabVIEW (National Instruments, TX). The angular position of the dimeric probe was analyzed by an algorithm based on a principal component analysis of the probe image.

We used a laboratory-made autofocus system to keep the probe in focus with a stepping motor (Oriental motor, Japan) rotating a focus knob.

We observed 8 molecules for [ATP] = [ADP] = 0.08  $\mu$ M, 9 molecules for [ATP] = [ADP] = 0.4  $\mu$ M, 8 molecules for [ATP] = [ADP] = 2  $\mu$ M, 8 molecules for [ATP] = [ADP] = 10  $\mu$ M, 9 molecules for [ATP] = [ADP] = 50  $\mu$ M, and 9 molecules for [ATP] = [ADP] = 250  $\mu$ M.

We applied an external torque on the probe attached to F<sub>1</sub> by using electrorotation method as described in [2]

### D. Numerical calculation

We first obtained the probability distribution of  $\theta$  and  $n$  at the steady state  $P^{\text{st}}(\theta, n)$  by numerically solving a master equation of the TASAM. The master equation of the TASAM is written as

$$\begin{aligned} \frac{\partial P_t(\theta, n)}{\partial t} = & -\frac{\partial}{\partial \theta} \left[ \frac{1}{\Gamma} \left( N_{\text{ex}} - \frac{\partial U_n(\theta)}{\partial \theta} \right) P_t(\theta, n) - \frac{k_B T}{\Gamma} \frac{\partial P_t(\theta, n)}{\partial \theta} \right] \\ & + R_{n-1}^+(\theta) P_t(\theta, n-1) + R_{n+1}^-(\theta) P_t(\theta, n+1) - [R_n^+(\theta) + R_n^-(\theta)] P_t(\theta, n). \end{aligned} \quad (\text{S1})$$

Since  $P^{\text{st}}(\theta, n)$  satisfies translational symmetry  $P^{\text{st}}(\theta, n) = P^{\text{st}}(\theta + 120^\circ, n+1)$ , we simplified Eq. (S1) by imposing the same translational symmetry on  $P_t(\theta, n)$  as

$$\begin{aligned} \frac{\partial P_t(\theta, 0)}{\partial t} = & -\frac{\partial}{\partial \theta} \left[ \frac{1}{\Gamma} \left( N_{\text{ex}} - \frac{\partial U_0(\theta)}{\partial \theta} \right) P_t(\theta, 0) - \frac{k_B T}{\Gamma} \frac{\partial P_t(\theta, 0)}{\partial \theta} \right] \\ & + R_0^+(\theta + 120^\circ) P_t(\theta + 120^\circ, 0) + R_0^-(\theta - 120^\circ) P_t(\theta - 120^\circ, 0) - [R_0^+(\theta) + R_0^-(\theta)] P_t(\theta, 0). \end{aligned} \quad (\text{S2})$$

We introduced reflecting boundaries at  $\theta_b^+$  and  $\theta_b^-$ , and discretized angular space with an interval  $\Delta\theta = 0.5^\circ$ . Then, we obtained  $P^{\text{st}}(\theta, 0)$  by evolving  $P_t(\theta, 0)$  using Euler method with the temporal interval  $\Delta t = 10^{-8}$  s or  $10^{-9}$  s.

The rotational rate  $V$  was evaluated from  $P^{\text{st}}(\theta, 0)$  as follows.  $V$  is related with a probability current in  $\theta$ -direction at the steady state

$$J_\theta^{\text{st}} = \sum_{n=-\infty}^{\infty} \left[ \frac{1}{\Gamma} \left( N_{\text{ex}} - \frac{\partial U_n(\theta)}{\partial \theta} \right) P^{\text{st}}(\theta, n) - \frac{k_B T}{\Gamma} \frac{\partial P^{\text{st}}(\theta, n)}{\partial \theta} \right], \quad (\text{S3})$$

as  $V = J_\theta^{\text{st}}/3$ . Then, we evaluated  $J_\theta^{\text{st}}$  by rewriting Eq. (S3) as

$$J_\theta^{\text{st}} = \sum_{n=-\infty}^{\infty} \left[ \frac{1}{\Gamma} \left( N_{\text{ex}} - \frac{\partial U_0(\theta - n \cdot 120^\circ)}{\partial \theta} \right) P^{\text{st}}(\theta - n \cdot 120^\circ, 0) - \frac{k_B T}{\Gamma} \frac{\partial P^{\text{st}}(\theta - n \cdot 120^\circ, 0)}{\partial \theta} \right], \quad (\text{S4})$$

and converted it to  $V$ .

The switching angle distribution is defined as  $\Lambda_n(\theta) = R_n^+(\theta) P^{\text{st}}(\theta, n) - R_{n+1}^-(\theta) P^{\text{st}}(\theta, n+1)$ . We evaluated  $\Lambda_0(\theta)$  as

$$\Lambda_0(\theta) = R_0^+(\theta) P^{\text{st}}(\theta, 0) - R_0^-(\theta - 120^\circ) P^{\text{st}}(\theta - 120^\circ, 0). \quad (\text{S5})$$

$\Lambda_n(\theta)$  may be obtained as  $\Lambda_n(\theta) = \Lambda_0(\theta - n \cdot 120^\circ)$  from the translational symmetry.

- 
- [1] Y. Rondelez, G. Tresset, T. Nakashima, Y. Kato-Yamada, H. Fujita, S. Takeuchi, and H. Noji, *Nature* **433**, 773 (2005).  
 [2] Y. Nakayama and S. Toyabe, *Phys. Rev. Lett.* **126**, 208101 (2021).
